# Supplementary material for: Allocation Problems in Ride-Sharing Platforms: Online Matching with Offline Reusable Resources
Source: arXiv:1711.08345 source file (2017-12-11)
Supplement: Supplementary file 1 [file 7_appendix.tex]

\section{Technical Lemmas}
In our main section, our algorithm for \kcspip uses the following version of the Chernoff-Hoeffding bounds. This can be easily derived from the standard form and we give a proof here for completeness.

\begin{theorem}[Chernoff bounds]
	\label{appx:chernoff}
	Let $X_1, X_2, \ldots, X_n \in [0,1]$ be independent random variables, satisfying the following $\mathbb{E}[\sum_{i}X_i] \leq \frac{c_1}{k}$ for some large $k$ and constant $c_1$. Then,
	
	$$\Pr[\sum_{i}X_i \geq c_2] \leq \left( \frac{c_1 e}{k c_2} \right) ^{c_2}$$
\end{theorem}

\begin{proof}
	We know that, $\Pr[\sum_{i} X_i \geq (1+ \delta)\mu] \leq \left( \frac{e^{\delta}}{(1+\delta)^{(1+\delta)}} \right)^{\mu}$ \\
	
	Note that we want $(1+\delta)(c_1/k) = c_2$, hence giving $1+\delta = \frac{kc_2}{c_1}$. Plugging this above, we get the desired bound.
\end{proof}

\begin{lemma}[Convexity]\label{lem:hm-convex}
	Assume $f:[0,1] \rightarrow [0,1]$ and it has second derivatives over $[0,1]$. Then we have that $\ln(1-t f(x))$ is a convex function of $x\in [0,1]$ for any given $t\in (0,1)$ iff $(1-f)(-f'') \ge f'^2$ for all $x \in [0,1]$. 
\end{lemma}
\begin{proof}
	Consider a given $t \in (0,1)$ and let $F(x)=\ln(1-t f(x))$. $F(x)$ is convex over $[0,1]$ iff $F'' \ge 0$ for all $x \in [0,1]$. We can verify that it is equivalent to the condition that $(1-f)(-f'') \ge f'^2$ for all $x \in [0,1]$.
\end{proof}
